# Supplementary material for: Observation of the spin Nernst effect
Source: arXiv:1607.02277 ancillary file (2017-06-01)
Supplement: Supplementary file 1 [file supplementary_material.pdf]

# Observation of the spin Nernst effect (Supplementary Information)

**S. Meyer[1,2], Y.-T. Chen[3,4], S. Wimmer[5], M. Althammer[1], T. Wimmer[1,2], R. Schlitz[1,6,7], S. Geprägs[1], H. Huebl[1,2,8], D. Ködderitzsch[5], H. Ebert[5], G.E.W. Bauer[3,9,10], R. Gross[1,2,8] and S.T.B. Goennenwein[1,2,6,7,8]**

1. Walther-Meißner-Institut, Bayerische Akademie der Wissenschaften, Walther-Meißner-Straße 8, 85748 Garching, Germany
2. Physik-Department, Technische Universität München, 85748 Garching, Germany
3. Kavli Institute of NanoScience, Delft University of Technology, Lorentzweg 1, 2628 CJ Delft, The Netherlands
4. RIKEN Center for Emergent Matter Science (CEMS), 2-1 Hirosawa, Wako, Saitama 351-0198, Japan
5. Department Chemie, Physikalische Chemie, Universität München, Butenandtstraße 5-13, 81377 München, Germany
6. present address: Institut für Festkörperphysik, Technische Universität Dresden, 01062 Dresden, Germany
7. present address: Center for Transport and Devices of Emergent Materials, Technische Universität Dresden, 01062 Dresden, Germany
8. Nanosystems Initiative Munich (NIM), Schellingstraße 4, 80799 München, Germany
9. Institute for Materials Research, Tohoku University, Sendai, Miyagi 980-8577, Japan
10. WPI Advanced Institute for Materials Research, Tohoku University, Sendai 980-8577, Japan

May 24, 2017

# 1 Supplementary Information (SI)

## 1.1 Theory of the spin Nernst magnetothermopower

Here we present a theoretical analysis of the SMT effect in N|FMI bilayer systems in terms of a non-equilibrium proximity effect caused by the simultaneous action of the spin Nernst effect (SNE) and the inverse spin Hall effect (ISHE). This effect scales like the product of the spin Hall and spin Nernst angle, and is modulated by the magnetization direction in YIG via the spin transfer at the N|FMI interface. Our explanation is a generalization of that of the spin Hall magnetoresistance [1, 2], and is based on the spin-diffusion approximation in the N layer in the presence of spin-orbit interaction [3] and quantum mechanical boundary conditions at the interface in terms of the spin-mixing conductance [4, 5].

We consider a N|FMI bilayer homogeneous in the x-y plane ($z = 0$ defines the interface), and calculate the spin accumulation, spin currents and finally the measured charge currents that are compared with the experimental SMT. We also find that the imaginary part of the spin-mixing conductance generates an anomalous Nernst effect (ANE) (that appears to be too small to be observable, however).

The spin current density in the weakly relativistic limit

$$\mathbf{j}_{\mathrm{s}} = -en\frac{< \mathbf{v} \times \boldsymbol{\sigma} + \boldsymbol{\sigma} \times \mathbf{v} >}{2} = (\mathbf{j}_{\mathrm{s,x}}, \mathbf{j}_{\mathrm{s,y}}, \mathbf{j}_{\mathrm{s,z}})^{\mathrm{T}} = (\mathbf{j}_{\mathrm{s}}^{\mathrm{x}}, \mathbf{j}_{\mathrm{s}}^{\mathrm{y}}, \mathbf{j}_{\mathrm{s}}^{\mathrm{z}}) \tag{1}$$

is a second-order tensor (in units of the charge current density $\mathbf{j}_{\mathrm{c}} = -en < \mathbf{v} >$), where $-e$ ($e > 0$) is the electron charge, $n$ is the density of the electrons, $\mathbf{v}$ is the velocity operator, $\boldsymbol{\sigma}$ is the vector of Pauli spin matrices, and $< ... >$ denotes the thermodynamic expectation value for a non-equilibrium state. The row vectors $\mathbf{j}_{\mathrm{s,i}} = -en < \mathbf{v} \times \sigma_{\mathrm{i}} + \sigma_{\mathrm{i}} \times \mathbf{v} > /2$ are the spin current densities polarized in the $\mathbf{i}$ direction, while the column vectors $\mathbf{j}_{\mathrm{s}}^{\mathrm{j}} = -en < v_{\mathrm{j}} \times \boldsymbol{\sigma} + \boldsymbol{\sigma} \times v_{\mathrm{j}} > /2$ denote the spin current densities with polarization $\eta$ flowing in the $\mathbf{j}$ direction. On the other hand, the heat current reads $\mathbf{j}_{\mathrm{h}} = n < (E - E_{\mathrm{F}})\mathbf{v} >$, where $E$ stands for the energy of the particle, $E_{\mathrm{F}}$ represents the Fermi energy. Ohm‘s Law for metals with spin-orbit interactions can be summarized by the relation between thermodynamic driving forces and currents that reflects the Onsager

reciprocity by the symmetry of the response matrix [2, 3]

$$\begin{pmatrix} \mathbf{j}_{\mathrm{c}} \\ \mathbf{j}_{\mathrm{h}} \\ \mathbf{j}_{\mathrm{s,x}} \\ \mathbf{j}_{\mathrm{s,y}} \\ \mathbf{j}_{\mathrm{s,z}} \end{pmatrix} = \sigma \begin{pmatrix} 1 & ST & \theta_{\mathrm{SH}}\mathbf{x}\times & \theta_{\mathrm{SH}}\mathbf{y}\times & \theta_{\mathrm{SH}}\mathbf{z}\times \\ ST & L_0T^2 & ST\theta_{\mathrm{SN}}\mathbf{x}\times & ST\theta_{\mathrm{SN}}\mathbf{y}\times & ST\theta_{\mathrm{SN}}\mathbf{z}\times \\ \theta_{\mathrm{SH}}\mathbf{x}\times & ST\theta_{\mathrm{SN}}\mathbf{x}\times & 1 & 0 & 0 \\ \theta_{\mathrm{SH}}\mathbf{y}\times & ST\theta_{\mathrm{SN}}\mathbf{y}\times & 0 & 1 & 0 \\ \theta_{\mathrm{SH}}\mathbf{z}\times & ST\theta_{\mathrm{SN}}\mathbf{z}\times & 0 & 0 & 1 \end{pmatrix} \begin{pmatrix} \nabla\mu_0/e \\ -\nabla T/T \\ \nabla\mu_{\mathrm{sx}}/(2e) \\ \nabla\mu_{\mathrm{sy}}/(2e) \\ \nabla\mu_{\mathrm{sz}}/(2e) \end{pmatrix} \tag{2}$$

where $\boldsymbol{\mu}_{\mathrm{s}} = (\mu_{\mathrm{sx}}, \mu_{\mathrm{sy}}, \mu_{\mathrm{sz}})^T - \mu_0\mathbf{1}$ is the spin accumulation, i.e. the spin-dependent chemical potential relative to the electrochemical potential $\mu_0$, $\sigma$ is the electrical conductivity, $S = -eL_0T\partial_E(\ln(\sigma))|_{E_F}$ is the Seebeck coefficient, $L_0 = (\pi^2/3)(k_{\mathrm{B}}/e)^2$ is the Lorenz number with $k_{\mathrm{B}}$ the Boltzmann constant, $\theta_{\mathrm{SH}}$ ($\theta_{\mathrm{SN}}$) is the spin Hall (Nernst) angle, and $\times$ denotes the vector cross product operating on the driving forces. The spin Hall (Nernst) effect [6, 7] is represented by the lower non-diagonal elements that generate the spin currents in the presence of an applied electric field (temperature gradient), while the inverse spin Hall (Nernst) effect is governed by elements above the diagonal that connect the gradients of the spin accumulations to the charge (heat) current density. The Mott relations, expressing the response to a temperature gradient in terms of the energy derivative of the electric response (as done above for the Seebeck coefficient), are the leading terms in the Sommerfeld expansion of the linear response coefficients given by Eqns. (20) and (21). They are exact in the limit of sufficiently low temperatures. Deviations from the Mott relations at elevated temperatures can be parameterized by a temperature-dependent effective Lorenz number. The ab-initio calculations detailed below, however, do not make use of the Sommerfeld approximation. In this study, we focus on the charge current generated by an external temperature gradient and thus the driving force is chosen to be a temperature gradient in the $\mathbf{x}$ direction $\nabla T = \mathbf{x}\partial_x T$ which drives a charge current $j_{c0}\mathbf{x} = -\sigma S\partial_x T\mathbf{x}$ via the Seebeck effect.

The spin accumulation $\mu_{\mathrm{s}}$ is obtained from the spin-diffusion equation in the normal metal

$$\nabla^2\boldsymbol{\mu}_{\mathrm{s}} = \frac{\boldsymbol{\mu}_{\mathrm{s}}}{\lambda^2} \tag{3}$$

where the spin-diffusion length $\lambda = \sqrt{D\tau_{\mathrm{sf}}}$ is expressed in terms of the charge diffusion constant $D$ and spin-flip relaxation time $\tau_{\mathrm{sf}}$ [8]. For films with thickness $t_{\mathrm{N}}$ in the $\mathbf{z}$ direction,

$$\boldsymbol{\mu}_{\mathrm{s}}(z) = \mathbf{A}e^{-z/\lambda} + \mathbf{B}e^{z/\lambda} \tag{4}$$

where the constant column vectors $\mathbf{A}$ and $\mathbf{B}$ are determined by the boundary

conditions at the interfaces. According to Eq. (2), the spin current in N consists of diffusion and spin Nernst drift contributions. Since our system is homogeneous in the x-y plane, we focus on the spin current density flowing in the $\mathbf{z}$ direction,

$$\mathbf{j}_\mathrm{s}^\mathrm{z}(z) = \frac{\sigma}{2e}\partial_z \boldsymbol{\mu}_\mathrm{s} - j_\mathrm{s0}^\mathrm{SN}\mathbf{y}, \tag{5}$$

where $j_\mathrm{s0}^\mathrm{SN} = -\theta_\mathrm{SN}\sigma S\partial_x T$ is the bare spin Nernst current, i.e., the spin current generated directly by the SNE. The boundary conditions require that $\mathbf{j}_\mathrm{s}^\mathrm{z}$ is continuous at the interfaces $z = t_\mathrm{N}$ and $z = 0$. The spin current at a vacuum (V) interface vanishes, $\mathbf{j}_\mathrm{s}(V) = 0$. The spin current density $\mathbf{j}_\mathrm{s}^{(\mathrm{F})}$ at a magnetic interface is governed by the spin accumulation and spin-mixing conductance:[4]

$$e\mathbf{j}_\mathrm{s}^{(\mathrm{F})}(\mathbf{m}) = G_\mathrm{r}\mathbf{m}\times(\mathbf{m}\times\boldsymbol{\mu}_\mathrm{s}) + G_\mathrm{i}(\mathbf{m}\times\boldsymbol{\mu}_\mathrm{s}) \tag{6}$$

where $\mathbf{m} = (m_x, m_y, m_z)^T$ is a unit vector along the magnetization and $G = G_\mathrm{r} + \imath G_\mathrm{i}$ the complex spin-mixing interface conductance per unit area and $\imath = \sqrt{-1}$. The imaginary part $G_\mathrm{i}$ can be interpreted as an effective exchange field acting on the spin accumulation. A positive current in Eq. (6) corresponds to up spins flowing from the FMI towards N. With these boundary conditions we determine the coefficients $\mathbf{A}$ and $\mathbf{B}$, which leads to the spin accumulation in the bilayer system

$$\boldsymbol{\mu}_\mathrm{s}(z) = \mathbf{y}\mu_s^0\frac{\sinh\frac{2z-t_\mathrm{N}}{2\lambda}}{\sinh\frac{t_\mathrm{N}}{2\lambda}} - \mathbf{j}_\mathrm{s}^{(\mathrm{F})}(\mathbf{m})\frac{2e\lambda}{\sigma}\frac{\cosh\frac{z-t_\mathrm{N}}{\lambda}}{\sinh\frac{t_\mathrm{N}}{\lambda}} \tag{7}$$

where $\mu_s^0 = (2e\lambda/\sigma)\mathbf{j}_\mathrm{s0}^\mathrm{SN}\tanh(t_\mathrm{N}/2\lambda)$ is the spin accumulation at the interface in the absence of spin transfer, i.e., when $G = 0$. Following Ref. [2], the spin accumulation reads

$$\begin{aligned}\frac{\boldsymbol{\mu}_\mathrm{s}(z)}{\mu_\mathrm{s}^0} &= \mathbf{y}\frac{\sinh\frac{2z-t_\mathrm{N}}{2\lambda}}{\sinh\frac{t_\mathrm{N}}{2\lambda}} \\ &\quad - [\mathbf{m}\times(\mathbf{m}\times\mathbf{y})\mathrm{Re} + (\mathbf{m}\times\mathbf{y})\mathrm{Im}]\frac{2\lambda G}{\sigma + 2\lambda G\coth\frac{t_\mathrm{N}}{\lambda}}\frac{\cosh\frac{z-t_\mathrm{N}}{\lambda}}{\sinh\frac{t_\mathrm{N}}{\lambda}}\end{aligned} \tag{8}$$

which leads to the distributed spin current in the N

$$\frac{\mathbf{j}_\mathrm{s}^z(z)}{j_\mathrm{s0}^\mathrm{SN}} = \mathbf{y}\frac{\cosh\frac{2z-t_\mathrm{N}}{2\lambda} - \cosh\frac{t_\mathrm{N}}{2\lambda}}{\cosh\frac{t_\mathrm{N}}{2\lambda}} - \left[\mathbf{m}\times(\mathbf{m}\times\mathbf{y})\mathrm{Re} + (\mathbf{m}\times\mathbf{y})\mathrm{Im}\right]\frac{2\lambda G\tanh\frac{t_\mathrm{N}}{2\lambda}}{\sigma + 2\lambda G\coth\frac{t_\mathrm{N}}{\lambda}}\frac{\sinh\frac{z-t_\mathrm{N}}{\lambda}}{\sinh\frac{t_\mathrm{N}}{\lambda}} \tag{9}$$

The ISHE drives a charge current in the x-y plane by the diffusion spin current component flowing along the **z** direction. The total longitudinal (along **x**) and transverse or Hall (along **y**) charge currents become

$$\frac{\mathbf{j}_\mathrm{c,long}(z)}{j_\mathrm{c0}} = 1 + \theta_\mathrm{SH}\theta_\mathrm{SN}\left[\frac{\cosh\frac{2z-t_\mathrm{N}}{2\lambda}}{\cosh\frac{t_\mathrm{N}}{2\lambda}} + (1-m_y^2)\mathrm{Re}\frac{2\lambda G\tanh\frac{t_\mathrm{N}}{2\lambda}}{\sigma + 2\lambda G\coth\frac{t_\mathrm{N}}{\lambda}}\frac{\sinh\frac{z-t_\mathrm{N}}{\lambda}}{\sinh\frac{t_\mathrm{N}}{\lambda}}\right] \tag{10}$$

$$\frac{\mathbf{j}_\mathrm{c,trans}(z)}{j_\mathrm{c0}} = \theta_\mathrm{SH}\theta_\mathrm{SN}(m_x m_y\mathrm{Re} - m_z\mathrm{Im})\frac{2\lambda G\tanh\frac{t_\mathrm{N}}{2\lambda}}{\sigma + 2\lambda G\coth\frac{t_\mathrm{N}}{\lambda}}\frac{\sinh\frac{z-t_\mathrm{N}}{\lambda}}{\sinh\frac{t_\mathrm{N}}{\lambda}} \tag{11}$$

For an open-circuit configuration for the charge current, the observable in the experiment (thermal voltage) is expressed as an electric field $\mathbf{E}_\mathrm{th} = E_\mathrm{th,x}\mathbf{x} + E_\mathrm{th,y}\mathbf{y}$ which compensates $j_\mathrm{c,long}$ and $j_\mathrm{c,trans}$:

$$E_\mathrm{th,x} = \left[1 + \theta_\mathrm{SH}\theta_\mathrm{SN}\left[\frac{\cosh\frac{2z-t_\mathrm{N}}{2\lambda}}{\cosh\frac{t_\mathrm{N}}{2\lambda}} + (1-m_y^2)\mathrm{Re}\frac{2\lambda G\tanh\frac{t_\mathrm{N}}{2\lambda}}{\sigma + 2\lambda G\coth\frac{t_\mathrm{N}}{\lambda}}\frac{\sinh\frac{z-t_\mathrm{N}}{\lambda}}{\sinh\frac{t_\mathrm{N}}{\lambda}}\right]\right]S\partial_x T$$

$$E_\mathrm{th,y} = \theta_\mathrm{SH}\theta_\mathrm{SN}(m_x m_y\mathrm{Re} - m_z\mathrm{Im})\frac{2\lambda G\tanh\frac{t_\mathrm{N}}{2\lambda}}{\sigma + 2\lambda G\coth\frac{t_\mathrm{N}}{\lambda}}\frac{\sinh\frac{z-t_\mathrm{N}}{\lambda}}{\sinh\frac{t_\mathrm{N}}{\lambda}}S\partial_x T. \tag{12}$$

Averaging the electric field components along **x** and **y** over the film thickness $z$, we obtain

$$\overline{E_\mathrm{th,x}} = [S + \Delta S_0 + \Delta S_1(1-m_\mathrm{y}^2)]\partial_x T \tag{13}$$

$$\overline{E_\mathrm{th,y}} = (\Delta S_1 m_x m_y - \Delta S_2 m_z)\partial_x T \tag{14}$$

which includes

$$\Delta S_0 = S\theta_\mathrm{SH}\theta_\mathrm{SN}\frac{2\lambda}{t_\mathrm{N}}\tanh\frac{t_\mathrm{N}}{2\lambda} \tag{15}$$

$$\Delta S_1 = -S\theta_\mathrm{SH}\theta_\mathrm{SN}\frac{\lambda}{t_\mathrm{N}}\mathrm{Re}\frac{2\lambda G\tanh^2\frac{t_\mathrm{N}}{2\lambda}}{\sigma + 2\lambda G\coth\frac{t_\mathrm{N}}{\lambda}} \tag{16}$$

$$\Delta S_2 = -S\theta_{\mathrm{SH}}\theta_{\mathrm{SN}}\frac{\lambda}{t_{\mathrm{N}}}\mathrm{Im}\frac{2\lambda G\tanh^2\frac{t_{\mathrm{N}}}{2\lambda}}{\sigma + 2\lambda G\coth\frac{t_{\mathrm{N}}}{\lambda}} \tag{17}$$

$\Delta S_1$ (caused mainly by $G_r$) contributes to the SMT, while $\Delta S_2$ (caused mainly by $G_i$) contributes only when there is a magnetization component normal to the plane (anomalous Nernst effect).
The voltages detected in our experiments are linked to the electric field components in Eq. (13) via

$$V_{\mathrm{thermal}} = -\int \overline{E_{\mathrm{th,x}}}(\mathbf{x})d\mathbf{x} \tag{18}$$

Thus, the spin current generated by the SNE generates additional contributions $\Delta S_0$ and $\Delta S_1$ to the Seebeck coefficient. For longitudinal thermopower measurements, we therefore expect a magnetization orientation dependent contribution to $S$ and thus to the thermopower voltage $V_{\mathrm{thermal}}$ proportional to $\Delta S_1(1-m_{\mathrm{y}}^2)$. This is caused by the spin transport across the N|FMI interface described mainly by $G_r$. Comparing Eq. (13) with the longitudinal SMR (cf. Ref. [2]), we find the same magnetization orientation dependence proportional to $m_{\mathrm{y}}^2$. We thus expect that the SMT has a similar fingerprint as the SMR, with modulations in $V_{\mathrm{thermal}}$ when the magnetization of the FMI (the YIG) is rotated in planes spanned by $\mathbf{x}$ and $\mathbf{y}$ as well as in planes spanned by $\mathbf{z}$ and $\mathbf{y}$, while we expect no modulations in $V_{\mathrm{thermal}}$ when the magnetization of the FMI is rotated in ($\mathbf{x}$,$\mathbf{z}$) plane.

## 1.2 First principles description of the spin Nernst effect

In an independent theoretical effort, we derive the magnitude of the spin Hall and the spin Nernst angles in bulk platinum from first principles. Assuming a constant chemical potential and considering both an electric field $\mathbf{E}$ and a temperature gradient $\nabla T$ as generating forces for a spin-polarized current

$$J^{\mathrm{s}} = -e\mathcal{L}^{\mathrm{sc}}\mathbf{E} - \mathcal{L}^{\mathrm{sq}}\nabla T/T \tag{19}$$

the tensors $\mathcal{L}^{\mathrm{sc}}$ and $\mathcal{L}^{\mathrm{sq}}$ describe the response of the system under investigation. For a spin-polarization axis along $\mathbf{i}$, the spin current along $\mathbf{j}$, and the electric field along $\mathbf{k}$, with $\mathrm{i(j,k)} \in \{\mathrm{x,y,z}\}$, one obtains for the former

$$\mathcal{L}^{\mathrm{sc,i}}_{\mathrm{jk}}(T) = -\frac{1}{e}\int dE\,\sigma^{\mathrm{sc,i}}_{\mathrm{jk}}(E)D(E,E_F,T)\;, \tag{20}$$

with $D(E,E_F,T) = \left(-\frac{\partial f(E,E_F,T)}{\partial E}\right)$, $f(E,E_F,T)$ the Fermi function, $E_F$ the Fermi energy (or chemical potential of the electrons at $T = 0\,\mathrm{K}$), and the

energy-dependent spin conductivity $\sigma^{\mathrm{sc,i}}_{\mathrm{jk}}(E)$ at $T$. The latter is obtained by applying the Kubo-Bastin linear response formalism and an appropriate form of the spin current density operator [9, 10] in combination with the relativistic KKR (Korringa-Kohn-Rostocker) band structure method [11, 12, 13] and the alloy analogy model [14] to account for thermally-induced structural disorder.

In analogy to the relation between the transport coefficient $L^{\mathrm{cq}}_{\mathrm{jk}}(T)$ and the energy-dependent electrical conductivity $\sigma^{\mathrm{cc}}_{\mathrm{jk}}(E)$ [15], the temperature-dependent spin transport coefficient $\mathcal{L}^{\mathrm{sq,i}}_{\mathrm{jk}}(T)$ is expressed in terms of the energy-dependent spin conductivity $\sigma^{\mathrm{sc,i}}_{\mathrm{jk}}(E)$:

$$\mathcal{L}^{\mathrm{sq,i}}_{\mathrm{jk}}(T) = -\frac{1}{e}\int dE\,\sigma^{\mathrm{sc,i}}_{\mathrm{jk}}(E)\,D(E,E_F,T)\,(E-E_F)\;. \tag{21}$$

Considering a temperature gradient $\nabla T$ without an external electric field $\mathbf{E}$, the electric current density

$$\mathbf{j}^{\mathrm{c}} = -eL^{\mathrm{cc}}\mathbf{E} - L^{\mathrm{cq}}\nabla T/T \tag{22}$$

vanishes when open-circuit conditions are imposed. Equation (22) implies that an internal electric field

$$\mathbf{E} \;=\; -\frac{1}{eT}(L^{\mathrm{cc}})^{-1}L^{\mathrm{cq}}\nabla T = S\,\nabla T \tag{23}$$

compensates the charge imbalance induced by $\nabla T$, where $S$ is the thermo-(magneto-) electric tensor. The ratios $\mathcal{L}^{\mathrm{sc,i}}_{\mathrm{jk}}/L^{\mathrm{cc}}_{\mathrm{kk}} = \theta_{\mathrm{SH}}$, i.e. the spin Hall angle ($\theta_{\mathrm{SH}}$), and $\mathcal{L}^{\mathrm{sq,i}}_{\mathrm{jk}}/L^{\mathrm{cq}}_{\mathrm{kk}} = \theta_{\mathrm{SN}}$, i.e. the corresponding spin Nernst angle ($\theta_{\mathrm{SN}}$), express the efficiency of conversion of a longitudinal charge current density into a transverse spin current density, generated by an electric field or a temperature gradient, respectively (see Eq. (2)). Since the conversion of the $\mathbf{y}$-polarized spin current along $\mathbf{z}$, generated by the SNE, back into an electric field along $\mathbf{x}$ is expressed by the inverse spin Hall conductivity $\sigma'^{,\mathrm{y}}_{\mathrm{xz}} = \sigma^{\mathrm{y}}_{\mathrm{xz}} = -\sigma^{\mathrm{y}}_{\mathrm{zx}}$ (See Ref. [16]), the relevant (inverse) spin Hall angle $\theta_{\mathrm{SH}}$ is the ratio $\mathcal{L}^{\mathrm{sc,y}}_{\mathrm{xz}}/\mathcal{L}^{\mathrm{cc}}_{\mathrm{xx}} = -\mathcal{L}^{\mathrm{sc,y}}_{\mathrm{zx}}/\mathcal{L}^{\mathrm{cc}}_{\mathrm{xx}}$. The spin Nernst angle $\theta_{\mathrm{SN}}$ is given by $\mathcal{L}^{\mathrm{sq,y}}_{\mathrm{zx}}/\mathcal{L}^{\mathrm{cq}}_{\mathrm{xx}}$. Using Eq. (23) and the expressions for the electrical and thermoelectrical conductivities in terms of Eqs. (20) and (21), $\sigma_{\mathrm{xx}}$ ($\sigma^{\mathrm{y}}_{\mathrm{zx}}$) $= -eL^{\mathrm{cc}}_{\mathrm{xx}}$ ($-e\mathcal{L}^{\mathrm{sc,y}}_{\mathrm{zx}}$) and $\alpha_{\mathrm{xx}}$ ($\alpha^{\mathrm{y}}_{\mathrm{zx}}$) $= -\frac{1}{T}L^{\mathrm{cq}}_{\mathrm{xx}}$ ($-\frac{1}{T}\mathcal{L}^{\mathrm{sq,y}}_{\mathrm{zx}}$), their (temperature-dependent) ratio can be written as

$$\frac{\theta_{\mathrm{SH}}}{\theta_{\mathrm{SN}}}(T) = \frac{-\sigma^{\mathrm{y}}_{\mathrm{zx}}(T)}{\sigma_{\mathrm{xx}}(T)}\frac{\alpha_{\mathrm{xx}}(T)}{\alpha^{\mathrm{y}}_{\mathrm{zx}}(T)} = +S_{\mathrm{xx}}(T)\frac{\sigma^{\mathrm{y}}_{\mathrm{zx}}(T)}{\alpha^{\mathrm{y}}_{\mathrm{zx}}(T)}\;. \tag{24}$$

Following the notation of the previous section, $\sigma_{\mathrm{xx}}$ corresponds to $\sigma$ in Eq. (2), $-\sigma^{\mathrm{y}}_{\mathrm{zx}}$ to $\theta_{\mathrm{SH}}\sigma$, $\alpha_{\mathrm{xx}}$ to $-\sigma S$ and $\alpha^{\mathrm{y}}_{\mathrm{zx}}$ to $-\theta_{\mathrm{SN}}\sigma S$. The energy-dependent conductivities entering Eqs. (20) and (21) and the corresponding expressions for the longitudinal transport coefficients were calculated for a set of energy points $E$ around $E_F$ for each temperature $T$ accounting for the effect of uncorrelated lattice displacements via the alloy analogy model [13].

Figure 1 shows the calculated values of $\sigma_{\mathrm{xx}}(E)$ (top) and $\sigma^{\mathrm{y}}_{\mathrm{zx}}(E)$ (bottom) for $T = 200\,\mathrm{K}$ (blue pluses), $250\,\mathrm{K}$ (black triangles), and $300\,\mathrm{K}$ (red squares). The temperature-dependent Seebeck coefficient, spin Hall conductivity and spin Nernst conductivity subsequently obtained from these are shown in Fig. (2) at the top left, top right and bottom left, respectively.

They were calculated using the fitted $\sigma(E)$ curves from Fig. 1 in the integrands of Eqs. (20) and (21), i.e. without making use of the Sommerfeld approximation, which would lead to the Mott relations for the Seebeck coefficient and spin Nernst conductivity. Finally, the ratio of the spin Hall and the spin Nernst angle, expressed by the above quantities as in Eq. (24), is shown as a function of temperature in Fig. (2), bottom right. As can be seen, for the conventions and definitions chosen here, the two angles have opposite signs for the whole temperature range considered here and $\theta_{\mathrm{SN}}$ is larger than $\theta_{\mathrm{SH}}$ for $T > 210$ K.

## 1.3 Experimental methods

The sample used in this study is a YIG|Pt thin film heterostructure. YIG hereby stands for Yttrium Iron Garnet ($Y_3Fe_5O_{12}$). The 40 nm thick YIG layer was epitaxially grown on a 500 $\mu$m thick, single crystalline, (111)-oriented Gadolinium Gallium Garnet (GGG, $Gd_3Ga_5O_{12}$) substrate via pulsed laser deposition using a stoichiometric targets [17]. The deposition was carried out in an oxygen atmosphere of 25 $\mu$bar, with a laser energy density of $2\,\mathrm{J/cm^2}$ at the target, and a substrate temperature of 550 °C. The YIG layer is capped in-situ, without breaking the vacuum, with a 4.1 nm thick Pt layer via electron beam evaporation at room temperature. The thicknesses of the YIG and Pt layer were determined by high-resolution X-ray reflectometry (HR-XRR) to $t_{\mathrm{F}} = (40 \pm 2)\,\mathrm{nm}$ and $t_{\mathrm{N}} = (4.1 \pm 0.2)\,\mathrm{nm}$, respectively. High-resolution X-ray diffraction (HR-XRD) measurements confirmed the polycrystallinity of the Pt thin film and revealed no secondary phases.

After pre-characterization, the sample was patterned into a Hall bar structure with the additional on-chip heater strip as sketched in Fig. 3(a) via optical lithography and Ar ion beam milling. The Hall bar has a width of $w = 250\,\mu\mathrm{m}$, a length of $l = 3150\,\mu\mathrm{m}$ and a contact separation of $s = 625\,\mu\mathrm{m}$, the heating strip along $\mathbf{y}$ is $w_{\mathrm{h}} = 250\,\mu\mathrm{m}$ wide and $l_{\mathrm{h}} = 1175\,\mu\mathrm{m}$ long, the distance between

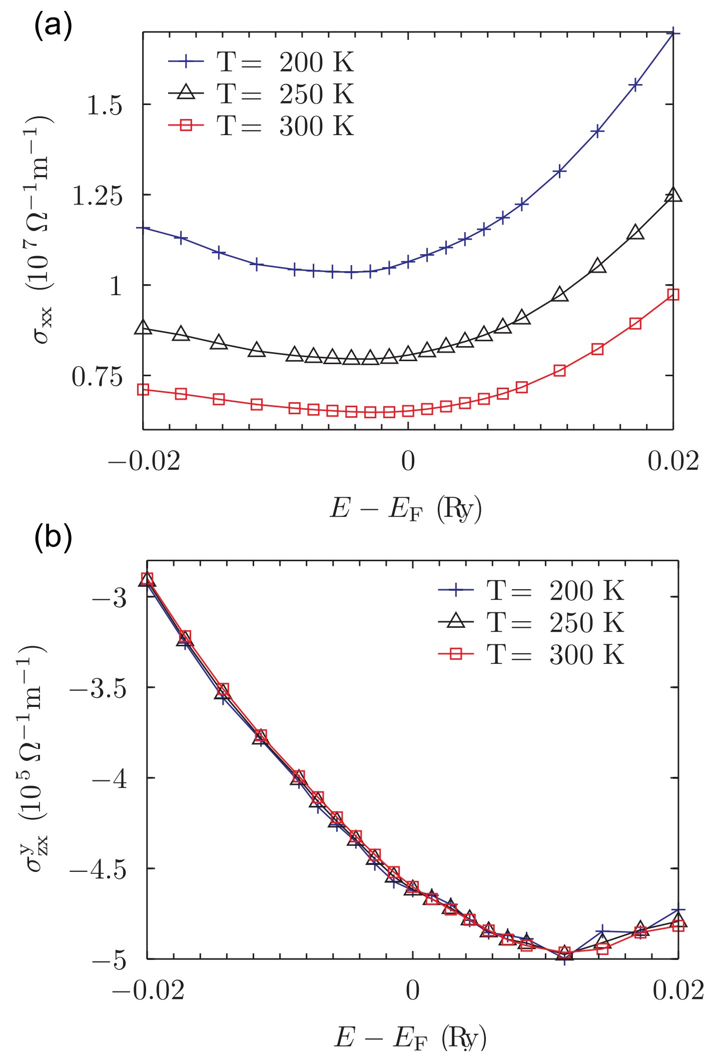


**Figure 1:** *Energy dependence of longitudinal charge (a) and transverse spin-polarized conductivity (b),* $\sigma_{\rm xx}(E)$ *and* $\sigma^{\rm y}_{\rm zx}(E)$*, respectively. Calculations were performed at fixed temperatures* $T = 200 - 300\,\rm K$ *in steps of* $10\,\rm K$ *using the alloy analogy model. Only the results for* $200\,\rm K$ *(blue pluses),* $250\,\rm K$ *(black triangles), and* $300\,\rm K$ *(red squares) are shown here.*

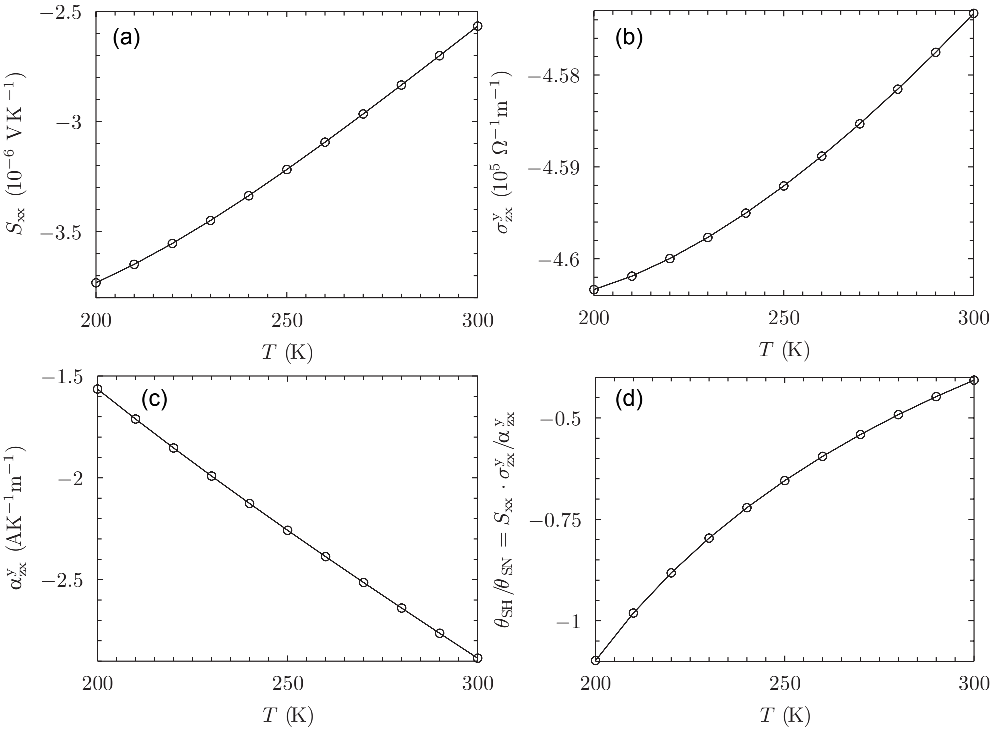


**Figure 2:** *Temperature dependence of* ***(a)*** *the Seebeck coefficient $S_{\mathrm{xx}}$,* ***(b)*** *the spin Hall conductivity $\sigma^{\mathrm{y}}_{\mathrm{zx}}$,* ***(c)*** *the spin Nernst conductivity, $\alpha^{\mathrm{y}}_{\mathrm{zx}}$, and* ***(d)*** *of the ratio $\theta_{\mathrm{SH}}/\theta_{\mathrm{SN}}$ as defined in Eq. (24).*

Hall bar and heating strip is $d = 250\,\mu$m. The sample is mounted onto a massive copper sample holder with one end, using GE 7031 thermally conductive varnish. The other end of the sample (with the heater strip) is connected to a Vespel block, again with GE varnish. In this way, the sample is thermally anchored to the sample holder on one end, and can be heated on the other, thermally 'isolated' end attached to the Vespel. All bonding pads at the Hall bar as well as the heater strip were connected to a printed circuit connector board with $30\,\mu$m thick Al wires via wedge bonding. The bonded sample is mounted on a dedicated magnet cryostat dipstick. This dipstick is enclosed in an evacuated steel jacket, such that the sample resides in vacuum. A pressure of $(5 \pm 1) \times 10^{-6}$ mbar within the sample space was kept constant during the experiments.

Our Oxford Instruments 3D vector magnet cryostat, equipped with a variable temperature insert (VTI), allows to apply magnetic fields $\leq 2\,$T in any desired orientation to the sample, while at the same time adjusting the VTI temperature

in the range $2\,\mathrm{K} \leq T \leq 300\,\mathrm{K}$. In all magneto-transport experiments discussed here, we used external magnetic field magnitudes $\mu_0 H_{\mathrm{ext}} \geq 500\,\mathrm{mT}$, which exceed the saturation magnetization $\mu_0 M_{\mathrm{Sat}}^{\mathrm{F}} \approx 170\,\mathrm{mT}$ of our YIG thin films at room temperature by at least about 3 times [18]. Thus, the magnetization vector $\mathbf{M}$ of the YIG layer is always aligned parallel to $\mu_0 \mathbf{H}_{\mathrm{ext}}$.

## On-chip thermometry

The base temperature of the sample holder (to which the cold end of the sample is anchored) was set to 220 K and stabilized using the PID feedback loop of a LakeShore LS340 temperature controller. Using the on-chip thermometry described below, we found that the temperature was stable within fluctuations of $\Delta T_{\mathrm{base}} = 3\,\mathrm{mK}$ (given by the temperature fluctuations displayed by the temperature controller) after a thermalization time of six hours. By applying heating currents of up to 20 mA to the heater strip next to the Hall bar by means of an Agilent B2900A Precision Source Measure Unit, corresponding to heating powers up to 286 mW, we created a temperature gradient along the Hall bar direction $\mathbf{x}$. The temperature profile along the Hall bar was determined by resistive thermometry (see Fig. 3) along two transverse Hall bar contact pairs separated by a distance of $l_1 = 2500\,\mu\mathrm{m}$ using two Keithley K2400 Source Measure Units and currents of $10\,\mu\mathrm{A}$ [cf. Fig. 3(a)]. In order to calibrate our 'on-chip Pt temperature sensors', we first stabilized the sample (viz the sample holder) temperature to 220 K (no heating current applied to the on-chip heater strip) and measured $R_{1,2}(T)$ at either end of the Hall bar while sweeping the sample temperature with 1 K/min up to 270 K using the temperature control of the dipstick just described. These resistance vs. temperature curves, shown in Fig. 3 (c) are used as calibration curves. After that, we again cooled the sample down to the base temperature of 220 K and determined $R_{1,2}(P_{\mathrm{heater}})$ while applying different heating powers up to 286 mW [cf. Fig. 3 (b)]. Comparing $R_{1,2}(P_{\mathrm{heat}})$ with the calibration curves taken before allow to recalculate the local sample temperature, such that a temperature profile of the sample with an experimental error of $\Delta T_{\mathrm{local}} \approx 0.4\,\mathrm{K}$ [see Fig. 3 (d)] is established. Please note that the error of $\Delta T_{\mathrm{local}} \approx 0.4\,\mathrm{K}$ is determined at the platinum strips by resistive thermometry , while the fluctuation $\Delta T_{\mathrm{base}} = 3\,\mathrm{mK}$ of the heat bath was determined by a Cernox temperature sensor at the sample holder.

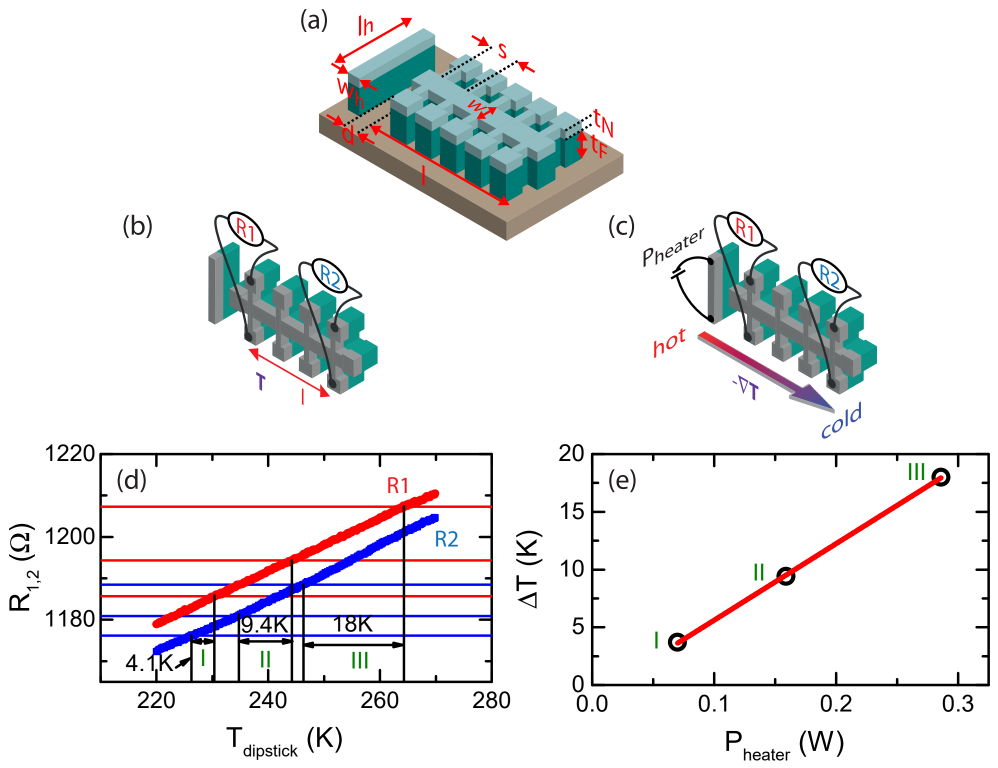


**Figure 3:** ***(a)*** *Experimental setup for SMT experiments. A YIG|Pt (*$t_\mathrm{F} = 40\,\mathrm{nm}/t_\mathrm{N} = 4.1\,\mathrm{nm}$*) thin film sample is patterned into a Hall bar geometry (width* $w = 250\,\mu\mathrm{m}$*, length* $l = 3150\,\mu\mathrm{m}$*). An additional heater strip (width* $w_\mathrm{h} = 250\,\mu\mathrm{m}$*, length* $l_\mathrm{h} = 1175\,\mu\mathrm{m}$*) is defined along* $\mathbf{y}$*, separated by* $d = 250\,\mu\mathrm{m}$ *beyond the top of the Hall bar.* ***(b,c)*** *Concept of the resistive thermometry: In a first step* ***(b)****, the resistance vs. temperature curves* $R_1(T)$ *and* $R_2(T)$ *along two transverse contact pairs are measured, while no power is applied to the heater. Here, the sample temperature is homogeneous and given by the dipstick temperature* $T_\mathrm{dipstick}$*.* $R_1(T)$ *and* $R_2(T)$ *serve as calibration curves for the thermometry. Afterwards* ***(c)****, the dipstick temperature is kept constant (*$T_\mathrm{base} = 220\,\mathrm{K}$*) while the electric power* $P_\mathrm{heater}$ *at the on-chip heater is increased stepwise.* $R_1$ *and* $R_2$ *are now taken as a function of* $P_\mathrm{heater}$*. Panel* ***(d)*** *shows both the calibration curves* $R_1(T)$ *and* $R_2(T)$ *and the heater dependent resistance values (horizontal lines). From those calibration curves, the local temperatures can be calculated as a function of* $P_\mathrm{heater}$*. Here, we show three different heater powers (I)* $P_\mathrm{heater} = 70\,\mathrm{mW}$*, (II)* $P_\mathrm{heater} = 159\,\mathrm{mW}$ *and (III)* $P_\mathrm{heater} = 286\,\mathrm{mW}$*. The extracted temperature differences* $\Delta T$ *along the Hall bar as a function of* $P_\mathrm{heater}$ *are shown in* ***(e)****.*

### Power scaling

We find a linear dependence of the temperature difference along the Hall bar on the applied heating power. Accordingly, we expect an almost linear scaling between thermopower and applied heater power [19]. The maximum generated temperature difference between the contacts separated by the distance $l_1$ was found to be 18.0 K for $P_{\mathrm{heater}} = 286\,\mathrm{mW}$. In Fig. 4, we show the thermopower voltage taken along the Hall bar direction for different, constant heating currents applied to the on-chip heater. Although the presence of a magnetic field usually is not required for the determination of the thermoelectric voltages, we applied a magnetic field of 1 T along $\mathbf{x}$ in theses experiments, in order to orient the magnetization of the YIG film and thus induce a reproducible contribution from the SMT. As evident from Fig. 4, we find an increase in the absolute value of $V_{\mathrm{thermal}}$ with increasing $I_{\mathrm{heater}}$, as expected for a thermopower effect from $V_{\mathrm{therm}} = S\Delta T$. For the highest heater current applied, we extract $S = -3.7\mu\mathrm{V/K}$ using $\Delta T = 18.0\,\mathrm{K}$. With respect to the average sample temperature $\bar{T} = (T_{\mathrm{hot}} - T_{\mathrm{cold}})/2 = 255.4\,\mathrm{K}$ extracted from the resistive thermometry shown above, $S$ is in excellent agreement with the literature value for Pt, $S(260\,\mathrm{K}) = -3.8\mu\mathrm{V/K}$ [19].

### Power modulation

To generate large temperature differences along the Hall bar, we use the on-chip heating strip consisting of the same YIG|Pt hybrid structure as the Hall bar. Since the YIG|Pt heterostructure shows spin Hall magnetoresistance (SMR) (i.e., a magnetization-orientation dependent resistance), a modulation of the heating power $P_{\mathrm{heater}} = R_{\mathrm{heater}} \times I_{\mathrm{heater}}^2$ with magnetization orientation must be taken into account. We measured the magnitude of the SMR effect in our sample to be $\Delta\rho_1/\rho_0 = (1.0 \pm 0.1) \times 10^{-3}$ at $T_{\mathrm{base}} = 220\,\mathrm{K}$ with $P_{\mathrm{heater}} = 286\,\mathrm{mW}$ applied to the heating strip. To avoid a SMR-based modulation of the heater power in our magnetization-orientation dependent thermopower measurements, we use a closed-loop control to adjust the applied heater current depending on magnetization orientation, such as to provide a constant heater power of $P_{\mathrm{heater}} = 286.30\,\mathrm{mW}$. Using this method, the applied heater power is stabilized with fluctuations smaller than 0.04 mW, see Fig. 5.

## 1.4 Fingerprint of the SMT

For SMT experiments, we remove all current sources from the Hall bar ($I_{\mathrm{q}} = 0$) and thermalize the sample to $T_{\mathrm{base}} = 220\,\mathrm{K}$. In order to apply a temperature

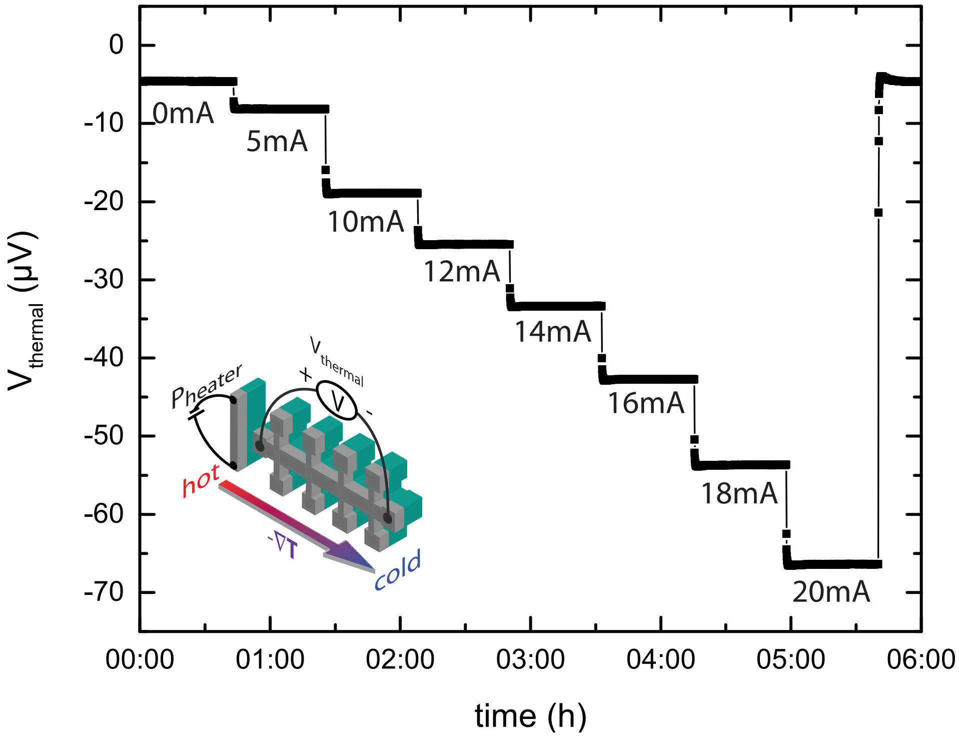


**Figure 4:** *Longitudinal thermal voltage $V_{\mathrm{thermal}}$ taken for a stepwise increase of currents applied to the heater strip.* $20\,\mathrm{mA}$ *correspond to* $P_{\mathrm{heater}} = 286\,\mathrm{mW}$.

gradient along $\mathbf{x}$ as a driving force, we bias the on-chip heater with the appropriate, magnetization orientation-dependent heater current, such that a constant heater power of $P_{\mathrm{heater}} = 286\,\mathrm{mW}$ independent of the magnetic field orientation is applied. We rotate a constant external magnetic field $\mu_0\mathbf{H}$ in the three orthogonal planes defined by $\mathbf{x}$, $\mathbf{y}$, and $\mathbf{z}$ and detect the longitudinal and transverse ($V_{\mathrm{thermal,trans}}$) voltages with an Agilent 34420A nanovoltmeter. We use a digital filter to detect the signal and average over 100 power line cycles using internal filter functions. We define the longitudinal $E_{\mathrm{thermal}} = -V_{\mathrm{thermal}}/l_{\mathrm{long}}$ and transverse $E_{\mathrm{thermal,trans}} = -V_{\mathrm{thermal,trans}}/l_{\mathrm{trans}}$ electric fields, where $l_{\mathrm{long}}$ and $l_{\mathrm{trans}}$ are the edge-to-edge separations of the contacts (Al-wire bonds) used for measuring $V_{\mathrm{thermal}}$ and $V_{\mathrm{thermal,trans}}$, respectively.

Figure 6 shows the evolution of $E_{\mathrm{thermal}}$ and $E_{\mathrm{thermal,trans}}$ as a function of the magnetization orientation while rotating the external magnetic field $\mu_0 H = 1\,\mathrm{T}$ and $0.5\,\mathrm{T}$ in in-plane (ip, $(\mathbf{x}, \mathbf{y})$-plane, panels d, g, j, and m), out-of-plane perpendicular $\mathbf{x}$ (oopx, $(\mathbf{y}, \mathbf{z})$-plane, panels e, h, k, and n) and out-of-plane

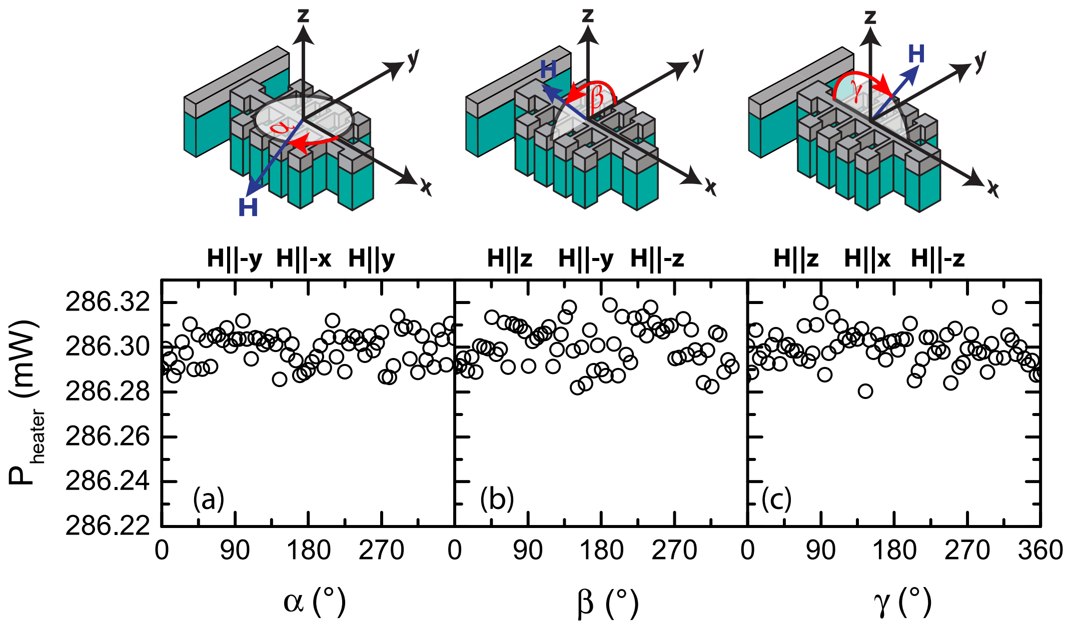


**Figure 5:** *Heater power $P_{\text{heater}}$ as a function of the YIG magnetization orientation in **(a)** ip, **(b)** oopx and **(c)** oopy configuration for $\mu_0 H = 1\,\text{T}$. During this measurement, we modulated the current $I_{\text{heater}}$ applied to the on-chip heater to keep the heating power constant.*

perpendicular $\mathbf{y}$ (oopy, $(\mathbf{x}, \mathbf{z})$-plane, panel f, i, l, and o) configuration. For the ip data of $E_{\text{thermal}}(1\ \text{T})$ [cf. Fig. 6(d),(j)], we find a $\sin^2\alpha$ dependence with $\Delta E_{\text{thermal}}(1\ \text{T}) \approx -30\,\mu\text{V/m}$, $\Delta E_{\text{thermal}}(0.5\ \text{T}) \approx -28\,\mu\text{V/m}$ on top of the thermopower signal given by the Seebeck effect of Pt. This modulation is smallest for $\mathbf{H} \parallel \mathbf{x}$ and $\mathbf{H} \parallel -\mathbf{x}$, and largest for $\mathbf{H} \parallel \mathbf{y}$ and $\mathbf{H} \parallel -\mathbf{y}$.

In the oopx rotation geometry [cf. Fig. 6(e),(k)], we find a similar, $\cos^2\beta$ modulation on top of the thermopower signal with an amplitude $\Delta E_{\text{thermal}}(1\ \text{T}) \approx -31\,\mu\text{V/m}$ and $\Delta E_{\text{thermal}}(0.5\ \text{T}) \approx -29\,\mu\text{V/m}$. Again, a maximum is recorded for $\mathbf{H} \parallel \mathbf{y}$ and $\mathbf{H} \parallel -\mathbf{y}$ and the signal level coincides in good approximation with the one found for the ip rotation. For this oopx geometry, the minima are located at $\mathbf{H} \parallel \mathbf{z}$ and $\mathbf{H} \parallel -\mathbf{z}$ and the voltage level for $\mathbf{H} \parallel \mathbf{z}$ is in good agreement with the signal detected at $\mathbf{H} \parallel \mathbf{x}$ in ip rotations.

For the oopy rotation [cf. Fig. 6(f),(l)], however, we find no angular dependence of $E_{\text{thermal}}$ within the noise level of our voltage measurement.

For the transverse thermopower signal $E_{\text{therm,trans}}$, we observe for the ip rotation plane a $\cos\alpha\sin\alpha$-dependence with a modulation amplitude $\Delta E_{\text{thermal,trans}}(1\ \text{T}) \approx -$

$40\,\mu$V/m and $\Delta E_{\text{thermal}}(0.5\text{ T}) \approx -39\,\mu$V/m, in good agreement with the modulation amplitude $\Delta E_{\text{thermal}}$ observed for the longitudinal thermopower and Eqs. (13),(14). As discussed in more detail below, the experimental data can be consistently fitted using one single value for $\Delta E_{\text{thermal}}$ and $\Delta E_{\text{thermal,trans}}$ ($E_1$ in Eqs. (25) and (26)). The additional magnetic field orientation independent background in $E_{\text{therm,trans}}$ can be attributed to a spurious longitudinal Seebeck signal caused by a small misalignment ($\approx 25\,\mu$m) of the two voltage probes on the Hall bar.

For the oopx and oopy rotation $E_{\text{therm,trans}}$ exhibits a sine dependence, that is dominated by the ordinary Nernst effect of Pt. A more detailed investigation of the field dependence of the modulation amplitude can identify the spin Nernst contributions in the spirit of Ref. [17].

The data sets shown in Fig. 6 and Fig. 3 in the main text can be understood in terms of the spin Nernst magneto-thermopower: In our geometry, the temperature gradient along $\mathbf{x}$ induces a spin Nernst spin current along $\mathbf{z}$ with spin polarization $\mathbf{s} \parallel \mathbf{y}$. Thus, $\mathbf{H} \parallel \mathbf{y}$ and $\mathbf{H} \parallel -\mathbf{y}$ correspond to the spin current open circuit boundary condition, since a spin transfer towards the YIG is prohibited for $\mathbf{H} \parallel \mathbf{s} \parallel \mathbf{y}$. On the other hand, both $\mathbf{H} \parallel \pm\mathbf{x}$ and $\mathbf{H} \parallel \pm\mathbf{z}$ correspond to perfect spin current short-circuit boundary conditions since they allow for a spin transfer. We compare the measurements with Eqs. (13),(14) in the theory section, by the red lines in Fig. 6 that represent a simulation for $E_{\text{therm}}$ and $E_{\text{therm,trans}}$ based on the following set of equations:

$$E_{\text{therm}} = E_0 - E_1 m_{\text{y}}^2, \tag{25}$$

$$E_{\text{therm,trans}} = E_{\text{off}} + E_1 m_x m_y - E_2 m_z, \tag{26}$$

and assuming that the magnetization $\mathbf{m}$ is always aligned parallel with the external applied magnetic field $\mathbf{H}$. The field-independent parameters $E_0 = 25.51$ mV/m, $E_1 = 42\ \mu$V/m, $E_{\text{off}} = 620\ \mu$V/m, $E_2 = 42\ \mu$V/m lead to an excellent agreement within the noise limit, such that the experimental set of data can completely be understood in the theoretical framework provided by the spin Nernst magnetothermopower. These findings thus leave little room for alternative explanations. We note that for the parameter $E_2$ a more systematic investigation in the spirit of Ref. [17] will be necessary to separate Spin Nernst contributions from additional effects like the ordinary Nernst effect.

Spurious effects can be ruled out by the observed angular dependence of the thermopower voltages. For example, $\nabla T$ along $\mathbf{z}$ drives a pure spin current along $\mathbf{z}$ with the spin polarization parallel to the magnetization direction of the YIG by the longitudinal spin Seebeck effect [20]. The inverse spin Hall

effect in Pt would generate a $\sin(\alpha)$ and $\cos(\beta)$ modulation of $E_{\mathrm{therm}}$ in the $(\mathbf{x}, \mathbf{y})$ and $(\mathbf{y}, \mathbf{z})$ rotation planes, while for $E_{\mathrm{therm,trans}}$ a $\cos(\alpha)$ and $\cos(\gamma)$ modulation would be present for the $(\mathbf{x}, \mathbf{y})$ and $(\mathbf{x}, \mathbf{z})$ rotation planes. This is not consistent with the observed angular dependence in the experiment. A temperature gradient along $\mathbf{y}$ would lead to a pure spin current flowing along $\mathbf{z}$ with the spin polarization parallel to the magnetization direction of the YIG because of the transversal spin Seebeck effect [21, 22]. The inverse spin Hall effect in Pt would then generate a $\sin(\alpha)$ and $\cos(\beta)$ modulation of $E_{\mathrm{therm}}$ and a $\cos(\alpha)$ and $\cos(\gamma)$ modulation of $E_{\mathrm{therm,trans}}$ in the $(\mathbf{x}, \mathbf{y})$, $(\mathbf{y}, \mathbf{z})$ and $(\mathbf{x}, \mathbf{y})$, $(\mathbf{x}, \mathbf{z})$ rotation planes, respectively, which is contradicted by the observations. Moreover, a magnon current driven by $\nabla T$ along $\mathbf{x}$ could lead to a pure spin current along $\mathbf{z}$ with a spin polarization parallel to $\mathbf{m}$ of YIG due to the magnon Hall effect [23]. Due to the inverse spin Hall effect in Pt this spin current will lead to a $\sin(\alpha)$ dependence of the longitudinal and a $\cos(\alpha)$ dependence of the transverse thermopower voltage in the $(\mathbf{x}, \mathbf{y})$ rotation plane. We do not observe such a modulation in our experiments. Taken together, spurious effects such as the ones mentioned above can be ruled out as the cause for the observed angular dependence of the thermopower signals.

## 1.5 Power and field dependence

On the same sample, we repeated the angle dependent magneto-thermopower measurements for different heating powers between 100 mW and 286 mW resulting in temperature differences between 7.7 K and 18.0 K along the Hall bar as well as for two different magnetic field strengths (0.5 T and 1 T). To extract the modulation amplitudes $\Delta V_{\mathrm{thermal}}$ and ratios $\Delta V_{\mathrm{thermal}}/V_{\mathrm{thermal}}$ from our experimental data, we performed $\cos^2\delta$ fits.

We observe an increase in the absolute value of the modulation voltage $\Delta V_{\mathrm{thermal}}$ with increasing $P_{\mathrm{heater}}$ in ip and oopx rotations. This is shown in Fig. 7(d) and (e) for two different magnetic field magnitudes. For both 0.5 T (red triangles) and 1 T (black squares), $\Delta V_{\mathrm{thermal}}$ increases with increasing $P_{\mathrm{heater}}$ and the difference between the 0.5 T and 1 T data points is within the experimental error of $\pm 5$ nV given by the thermal stability of the nanovoltmeters. As the SMT can be interpreted as a modulation on the thermal voltage due to a spin current flow across the YIG|Pt interface, the relative amplitude of the modulation of the longitudinal voltage is expected to be independent of both heating power $P_{\mathrm{heater}}$ and external magnetic field strength $\mu_0 H$, as long as a thermally driven spin current is generated. We find that, within the experimental error, the ratio is almost constant as a function of $P_{\mathrm{heater}}$ and $\mu_0 H$ for ip and oopx, $\Delta V_{\mathrm{thermal}}/V_{\mathrm{thermal}} \approx 1.2 \times 10^{-3}$. For the temperature range

studied here (the average sample temperature rises with increasing $P_{\mathrm{heater}}$, see Fig. 3), $\theta_{\mathrm{SH}}$ is known to be almost independent of temperature [24]. Considering $\Delta V_{\mathrm{thermal}}/V_{\mathrm{thermal}} \approx$ const., which is proportional to $\theta_{\mathrm{SH}}\theta_{\mathrm{SN}}$, the data in Fig. 7(d) and (e) suggest that the temperature dependence of the spin Nernst angle $\theta_{\mathrm{SN}}$ is rather weak.

The power dependence of the oopy signal is depicted in Fig. 7(f). As stated by Eq. (13), we expect a constant SMT signal as a function of the magnetization orientation in this geometry. While $\Delta V_{\mathrm{thermal}}$ scales with $P_{\mathrm{heater}}$ [cf. Fig. 7(d, e)] for ip and oopx rotations, we find that the modulation amplitude observed in oopy is almost constant [$\Delta V_{\mathrm{thermal}}^{\mathrm{oopy}} \approx -25\,\mathrm{nV}$, cf. Fig. 7(f)].Thus, the origin of the modulation in oopy rotations is not related to the spin Nernst magnetothermopower. However, this power independence can not be explained by the interpretation of $\Delta V_{\mathrm{thermal}}^{\mathrm{oopy}}$ with a non-vanishing $\mathbf{y}$ component of $\nabla T$. Additionally, $\Delta V_{\mathrm{thermal}}^{\mathrm{oopy}}$ seems to increase with increasing magnetic field strength. The decrease of $\Delta V_{\mathrm{thermal}}^{\mathrm{oopy}}(P_{\mathrm{heater}})$ also results in a negative power dependence of the voltage ratio $\Delta V_{\mathrm{thermal}}^{\mathrm{oopy}}/V_{\mathrm{thermal}}$. With increasing heater power, the voltage modulation in oopy decreases slightly. This again is at odds with the results found for ip and oopx rotations. In conclusion, due to the absence of a power dependence, the modulation of the thermal voltage in oopy rotations can neither be attributed to the SMT concept for $\nabla T \cdot \mathbf{y} \neq 0$, nor to parasitic thermopower effects.

## 1.6 Calculation of the spin Nernst angle

Now, we utilize the theory of Sec. 1.1 to extract the heat to spin conversion efficiency for Pt, i.e. the spin Nernst angle $\theta_{\mathrm{SN}}$. To this end, we calculate the relative thermopower ratio between open and short-circuit spin current boundary conditions,

$$\frac{\Delta V_{\mathrm{thermal}}}{V_{\mathrm{thermal}}} = \frac{V_{\mathrm{thermal}}(\mathbf{H} \parallel \mathbf{y}, \mathrm{open}) - V_{\mathrm{thermal}}(\mathbf{H} \perp \mathbf{y}, \mathrm{short})}{V_{\mathrm{thermal}}(\mathbf{H} \parallel \mathbf{y}, \mathrm{open})}. \tag{27}$$

Via Eq. (13), the definitions of $V_{\mathrm{thermal}}(\mathbf{H} \parallel \mathbf{y}, \mathrm{open})$ and $V_{\mathrm{thermal}}(\mathbf{H} \perp \mathbf{y}, \mathrm{short})$ read

$$V_{\mathrm{thermal}}(\mathbf{H} \parallel \mathbf{y}, \mathrm{open}) = -\left(S + \Delta S_0\right)\Delta T \tag{28}$$

and

$$V_{\mathrm{thermal}}(\mathbf{H} \perp \mathbf{y}, \mathrm{short}) = -\left(S + \Delta S_0 + \Delta S_1\right)\Delta T \tag{29}$$

with $\Delta T = T_{\mathrm{hot}} - T_{\mathrm{cold}} > 0$. Thus, $\Delta V_{\mathrm{thermal}}/V_{\mathrm{thermal}}$ corresponds to $-\Delta S_1/\tilde{S}$ with $\tilde{S} = S + \Delta S_0$.

We find $\Delta V_{\mathrm{thermal}}/V_{\mathrm{thermal}} = -100\,\mathrm{nV}/66.225\,\mu\mathrm{V} = -1.5 \times 10^{-3}$ from the raw

data taken at 1 T in the oopx plane shown in Fig. 3(f) in the main text. Based on Eq. (16), we calculate the spin Nernst angle $\theta_{\mathrm{SN}}$ via

$$\theta_{\mathrm{SN}} \approx -\frac{\Delta S_1}{S}\frac{t_{\mathrm{N}}}{\theta_{\mathrm{SH}}\lambda}\frac{\sigma_{\mathrm{N}} + 2\lambda G_r \coth\frac{t_{\mathrm{N}}}{\lambda}}{2\lambda G_r \tanh^2\frac{t_{\mathrm{N}}}{2\lambda}}. \tag{30}$$

We use $G_r = 4.0 \times 10^{14}\,\Omega^{-1}\mathrm{m}^{-2}$, $\lambda = 1.5\,\mathrm{nm}$ and $\theta_{\mathrm{SH}} = 0.11$ determined in Ref. [24] for YIG|Pt hybrids at $T = 250\mathrm{K}$ comparable to $\bar{T} = 255\mathrm{K}$ used in our thermopower measurements for this sample. With these parameters, we obtain $\theta_{\mathrm{SN}} = -0.20$ from Eq. (30).

It seems surprising that we are able to confirm the sign of the spin Nernst angle by transport experiments. Since SMR depends on the square of the spin Hall angle and cannot be used to measure its sign. Similarly, the SMT depends on the product of $\theta_{\mathrm{SN}}$ and $\theta_{\mathrm{SH}}$, so from these data alone we cannot conclude that $\theta_{\mathrm{SN}} < 0$. We come to our conclusion only because spin pumping measurements conclusively find a positive spin Hall angle in Pt [25]. We note that from a physical point of view $\theta_{\mathrm{SN}} < 0$ is not problematic at all. For $S < 0$, $\theta_{\mathrm{SN}} < 0$ corresponds to $\alpha^{\mathrm{y}}_{\mathrm{zx}} > 0$, i.e. the spin Nernst conductivity is positive. For $\theta_{\mathrm{SH}} > 0$, one finds $\sigma^{\mathrm{y}}_{\mathrm{xz}} > 0$ and accordingly due to Onsager symmetry $\sigma^{\mathrm{y}}_{\mathrm{zx}} < 0$. In the Sommerfeld limit ($T \to 0$) this implies that the spin Hall conductivity $\sigma^{\mathrm{y}}_{\mathrm{zx}}$ and its energy derivative at the Fermi energy, which is proportional to $\alpha^{\mathrm{y}}_{\mathrm{zx}}$, have the same sign, as $\theta_{\mathrm{SH}}$ represents the inverse spin Hall conductivity $\sigma^{\mathrm{y}}_{\mathrm{xz}} = -\sigma^{\mathrm{y}}_{\mathrm{zx}}$ and $\theta_{\mathrm{SN}}$ the (direct) spin Nernst conductivity $\alpha^{\mathrm{y}}_{\mathrm{zx}}$. Indeed, our first-principles calculations of the ratio between $\theta_{\mathrm{SH}}$ and $\theta_{\mathrm{SN}}$ find $\theta_{\mathrm{SH}}/\theta_{\mathrm{SN}} \approx -0.6$ at 250 K [see Sec. 1.2 and Fig. 2(d)]. This beautifully agrees with the ratio $\theta_{\mathrm{SH}}/\theta_{\mathrm{SN}} \approx -0.5$ found in our experiments.

## 1.7 Control Experiments

In the spirit of recent magnon-mediated magnetoresistance experiments [26, 27, 28, 29, 30, 31, 32], we conducted further control experiments to exclude spurious signals leading to the observed SMT. We investigated two samples: a GGG/YIG/Pt, and a GGG/Pt heterostructure. The GGG/YIG/Pt heterostructure was fabricated starting from a single crystalline (111) oriented GGG substrate onto which a 2 $\mu$m thick YIG film was deposited by liquid-phase epitaxy. After cleaning in a piranha solution, a 10 nm thick Pt film was deposited on the YIG film by electron beam evaporation [33]. For the second sample, we used a bare single crystalline (111) oriented GGG substrate, which also was cleaned in a piranha solution and then covered with a 5.8 nm

thick Pt film by electron beam evaporation. Subsequently, the Pt films on both samples were patterned into thin stripes using electron beam lithography and Argon ion beam milling, as described in more detail e.g. in Refs. [27, 28]. As sketched in Fig. 8(a), for the GGG/YIG/Pt heterostructure, the Pt strips had a width of $w_{\mathrm{N1}} = 0.5\ \mu$m and length of $l_{\mathrm{N1}} = 148\ \mu$m, both strips being separated by $d_{\mathrm{N1}} = 1.6\ \mu$m. For the GGG/Pt sample (see Fig. 8(b)), the strip dimensions were $w_{\mathrm{N2}} = 1\ \mu$m, $l_{\mathrm{N2}} = 148\ \mu$m, and $d_{\mathrm{N2}} = 2.6\ \mu$m. Both samples were mounted into the very same superconducting 3D-vector magnet cryostat, that was also used for the SMT experiments discussed in the main text, and cooled down to a sample temperature of $T_{\mathrm{base}} = 220$ K. For both samples a constant DC electrical current $I_{\mathrm{drive}}$ was applied to one strip by a Keithley 2400 current source, while the voltage $V_{\mathrm{nl}}$ across the other strip was recorded using a Keithley 2182A Nanovoltmeter. As detailed in [34, 26, 27], $I_{\mathrm{drive}}$, on one hand, generates a local thermal gradient owing to the Joule heating power $P_{\mathrm{heater}}$ associated with the charge current flow. The presence of this thermal gradient induces non-local thermopower voltages in the second Pt strip. On the other hand, when a magnetic insulator is located beneath the Pt strip, a non-equilibrium magnon population is injected into the magnet by virtue of the spin Hall spin accumulation. Magnon diffusion to the second Pt contact results in a non-local Ohmic voltage signal in the second strip, also called magnon-mediated magnetoresistance. We separate the non-local thermal and resistive contributions to $V_{\mathrm{nl}}$ by current reversal [35]: for each data point, the current polarity applied to the first strip is changed from positive ($+I_{\mathrm{drive}}$) to negative ($-I_{\mathrm{drive}}$) and the voltage signals $V_{\mathrm{nl}}(+I)$ and $V_{\mathrm{nl}}(-I)$ are recorded for the two different bias current polarities. The thermal voltage is then extracted as $V_{\mathrm{nl,therm}} = (V_{\mathrm{nl}}(+I) + V_{\mathrm{nl}}(-I))/2$, which is even with respect to current reversal. The MMR signal corresponds to $V_{\mathrm{nl,MMR}} = (V_{\mathrm{nl}}(+I) - V_{\mathrm{nl}}(-I))/2$. In the following, we concentrate on the thermal signal. We carried out SMT measurements for both samples with similar heater power and thermal gradients being present along $\mathbf{x}$. While the exact magnitude of the thermal gradient is difficult to quantify (the detector contact is very close to the "heater" and rather wide ($w \approx d$), such that it cannot be used for reasonable spatially resolved Pt thermometry), we find in SMT experiments in the oopy configuration that the ordinary Nernst signal recorded across the detector contact in the two samples is the same (to within 20 %).

In Fig. 8(c) we show the results obtained for the GGG/YIG/Pt sample for an external magnetic field of 1 T rotated in the $\mathbf{x} - \mathbf{y}$ plane and a heater power of 8.68 mW ($I = 1$ mA). $V_{\mathrm{nl,therm}}$ exhibits a clear $\cos(\alpha)$ dependence, which we attribute to a commonly observed spin Seebeck contribution due to a local thermal gradient along $\mathbf{z}$ [26, 29]. We fit the data with a cosine function for

both clockwise and counterclockwise rotations and extract an amplitude of $19.3\,\mu$V for the spin Seebeck signal. Subtracting the fitted $\cos\alpha$ function from the data we obtain the thermal voltage signal $\Delta V_{\mathrm{nl,therm}}$ plotted in Fig. 8(e). This signal exhibits the same angular dependence as the transverse spin Nernst thermopower signal in Fig. 6(g). We thus attribute this signal again to the SMT. Here, the modulation amplitude $\Delta V_{\mathrm{nl,therm}}$ is 0.15 $\mu$V, which corresponds to an electric field of 1 mV/m. This signal is much larger than the SMT signal observed in standard SMT experiments because the small spacing between heater and detector strip implies a much larger in-plane temperature gradient.

Repeating the thermopower experiments on the GGG/Pt sample, again using an external magnetic field of 1 T and a heater power of 12.2 mW, we obtain the results compiled in Fig. 8(d). For the GGG/Pt we do *not* observe any angular dependence of $V_{\mathrm{nl,therm}}$ for the ip geometry as expected considering that no SSE should be present in the absence of a magnetic insulator layer (for the oopx and oopy geometry we observe the ordinary Nernst effect of the Pt, as mentioned above). We subtract a (already small) constant voltage offset of 0.655 $\mu$V from $V_{\mathrm{nl,therm}}$ to obtain a $\Delta V_{\mathrm{nl,therm}}$. The result of this procedure is shown in Fig. 8(f) (on the same scale as for Fig. 8(e)). Again, there is no systematic angular dependence for $\Delta V_{\mathrm{nl,therm}}$ in the GGG/Pt sample. This shows that the presence of a magnetic insulator layer (YIG layer) is mandatory for the SMT to arise, as expected in the SNE picture proposed in the main manuscript. This control experiment thus further corroborates the notion that the SMT observed in YIG/Pt heterostructures indeed originates from the spin Nernst effect.

Taken together, the results compiled in Fig. 8 demonstrate that the SMT signal is only observed in YIG/Pt heterostructures while it is absent if only a GGG/Pt bilayer is used. Thus, these results further confirm our model predictions for the SMT and provide additional evidence for our first experimental observation of the spin Nernst effect. Moreover, these results show that the SMT is observable in non-local sample geometries, which broadens its appeal and relevance.

# References


[1] Nakayama, H., Althammer, M., Chen, Y.-T., Uchida, K., Kajiwara, Y., Kikuchi, D., Ohtani, T., Geprägs, S., Opel, M., Takahashi, S., Gross, R., Bauer, G. E. W., Goennenwein, S. T. B., and Saitoh, E. *Physical Review Letters* **110**, 206601 (2013).

[2] Chen, Y.-T., Takahashi, S., Nakayama, H., Althammer, M., Goennenwein, S. T. B., Saitoh, E., and Bauer, G. E. W. *Physical Review B* **87**, 144411 (2013).

[3] Takahashi, S., Imamura, H., and Maekawa, S. In *Concepts in Spin electronics,* Maekawa, S., editor, 343. Oxford University Press, New York (2006).

[4] Brataas, A., Bauer, G. E., and Kelly, P. J. *Physics Reports* **427**, 157 (2006).

[5] Jia, X., Liu, K., Xia, K., and Bauer, G. E. W. *Europhysics Letters* **96**, 17005 (2011).

[6] Borge, J., Gorini, C., and Raimondi, R. *Physical Review B* **87**,085309 (2013).

[7] Tölle, S., Gorini, C., and Eckern, U. *Physical Review B* **90**, 235117 (2014).

[8] Valet, T. and Fert, A. *Physical Review B* **48**, 7099 (1993).

[9] Vernes, A., Györffy, B. L., and Weinberger, P. *Physical Review B* **76**, 012408 (2007).

[10] Lowitzer, S., Gradhand, M., Ködderitzsch, D., Fedorov, D. V., Mertig, I., and Ebert, H. *Physical Review Letters* **106**, 056601 (2011).

[11] Butler, W. H. *Physical Review B* **31**, 3260 (1985).

[12] Banhart, J., Bernstein, R., Voitländer, J., and Weinberger, P. *Solid State Communications* **77**, 107 (1991).

[13] Ködderitzsch, D., Chadova, K., and Ebert, H. *Physical Review B* **92**, 184415 (2015).

[14] Ebert, H., Mankovsky, S., Chadova, K., Polesya, S., Minár, J., and Ködderitzsch, D. *Physical Review B* **91**,165132 (2015).

[15] Jonson, M. and Mahan, G. D. *Physical Review B* **21**, 4223 (1980).

[16] Seemann, M., Ködderitzsch, D., Wimmer, S., and Ebert, H. *Physical Review B* **92**, 155138 (2015).

[17] Althammer, M., Meyer, S., Nakayama, H., Schreier, M., Altmannshofer, S., Weiler, M., Huebl, H., Geprägs, S., Opel, M., Gross, R., Meier, D., Klewe, C., Kuschel, T., Schmalhorst, J.-M., Reiss, G., Shen, L., Gupta, A., Chen, Y.-T., Bauer, G. E. W., Saitoh, E., and Goennenwein, S. T. B. *Physical Review B* **87**, 224401 (2013).

[18] Geprägs, S., Meyer, S., Altmannshofer, S., Opel, M., Wilhelm, F., Rogalev, A., Gross, R., and Goennenwein, S. T. B. *Applied Physics Letters* **101**, 262407 (2012).

[19] Moore, J. P. and Graves, R. S. *Journal of Applied Physics* **44**, 1174 (1973).

[20] Uchida, K., Adachi, H., Ota, T., Nakayama, H., Maekawa, S., and Saitoh, E. *Applied Physics Letters* **97**, 172505 (2010).

[21] Uchida, K., Takahashi, S., Harii, K., Ieda, J., Koshibae, W., Ando, K., Maekawa, S., and Saitoh, E. *Nature* **455**, 778 (2008).

[22] Jaworski, C. M., Yang, J., Mack, S., Awschalom, D. D., Heremans, J. P., and Myers, R. C. *Nature Materials* **9**, 898 (2010).

[23] Onose, Y., Ideue, T., Katsura, H., Shiomi, Y., Nagaosa, N., and Tokura, Y. *Science* **329**, 297 (2010).

[24] Meyer, S., Althammer, M., Geprägs, S., Opel, M., Gross, R., and Goennenwein, S. T. B. *Applied Physics Letters* **104**, 242411 (2014).

[25] Czeschka, F. D., Dreher, L., Brandt, M. S., Weiler, M., Althammer, M., Imort, I.-M., Reiss, G., Thomas, A., Schoch, W., Limmer, W., Huebl, H., Gross, R., and Goennenwein, S. T. B. *Physical Review Letters* **107**, 046601 (2011).

[26] Cornelissen, L. J., Liu, J., Duine, R. A., Youssef, J. B., and van Wees, B. J. *Nature Physics* **11**, 1022 (2015).

[27] Goennenwein, S. T. B., Schlitz, R., Pernpeintner, M., Ganzhorn, K., Althammer, M., Gross, R., and Huebl, H. *Applied Physics Letters* **107**, 172405 (2015).

[28] Ganzhorn, K., Klingler, S., Wimmer, T., Geprägs, S., Gross, R., Huebl, H., and Goennenwein, S. T. B. *Applied Physics Letters* **109**, 022405 (2016).

[29] Cornelissen, L. J., Peters, K. J. H., Bauer, G. E. W., Duine, R. A., and van Wees, B. J. *Physical Review B* **94**,014412 (2016).

[30] Vélez, S., Bedoya-Pinto, A., Yan, W., Hueso, L. E., and Casanova, F. *Physical Review B* **94**,174405 (2016).

[31] Wu, H., Wan, C. H., Zhang, X., Yuan, Z. H., Zhang, Q. T., Qin, J. Y., Wei, H. X., Han, X. F., and Zhang, S. *Physical Review B* **93**,060403 (2016).

[32] Li, J., Xu, Y., Aldosary, M., Tang, C., Lin, Z., Zhang, S., Lake, R., and Shi, J. *Nature Communications* **7**, 10858 (2016).

[33] Pütter, S., Geprägs, S., Schlitz, R., Althammer, M., Erb, A., Gross, R., and Goennenwein, S. T. B. *Applied Physics Letters* **110**, 012403 (2017).

[34] Roschewsky, N., Schreier, M., Kamra, A., Schade, F., Ganzhorn, K., Meyer, S., Huebl, H., Geprägs, S., Gross, R., and Goennenwein, S. T. B. *Applied Physics Letters* **104**, 202410 (2014).

[35] Schreier, M., Roschewsky, N., Dobler, E., Meyer, S., Huebl, H., Gross, R., and Goennenwein, S. T. B. *Applied Physics Letters* **103**), 242404 (2013).

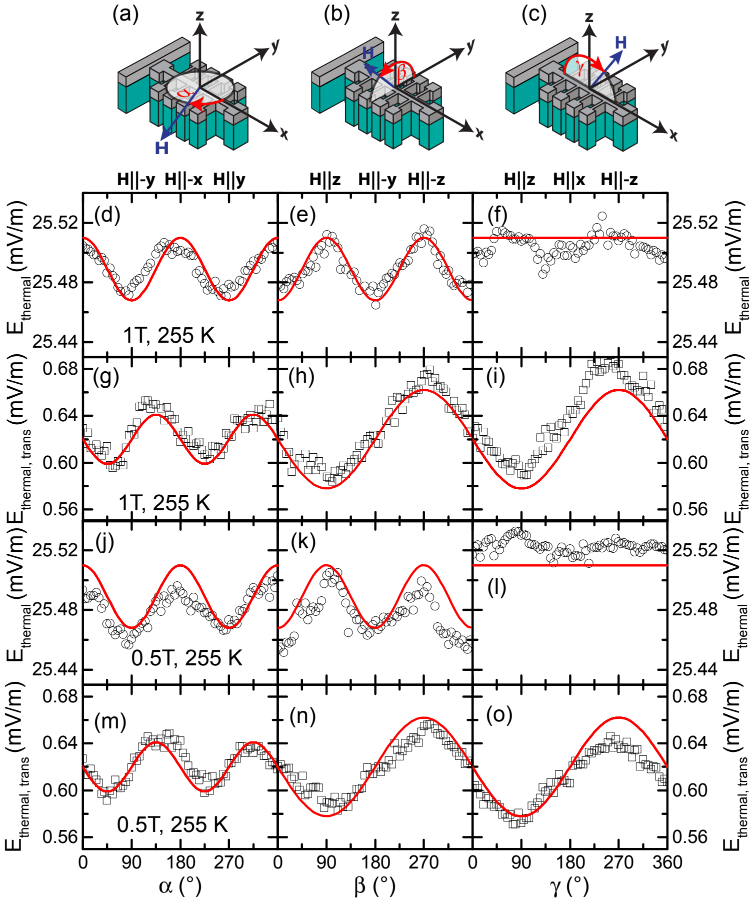


**Figure 6:** ***(a)-(c)*** *The magnetization vector* $\mathbf{M}$ *of the YIG layer is rotated by an external magnetic field in the three different rotation planes spanned by* ($\mathbf{x}$, $\mathbf{y}$) *(panel **(a)**),* ($\mathbf{y}$, $\mathbf{z}$)*(panel **(b)**) and* ($\mathbf{x}$, $\mathbf{z}$)*(panel **(c)**). The measured thermal electric field* $E_{\mathrm{thermal}}$ *(black circles) for all three geometries and* $P_{\mathrm{heater}} = 286\,\mathrm{mW}$ *(or* $\Delta T = 18.0\,\mathrm{K}$ *along the Hall bar) is depicted in panels **(d)**,**(j)** for the* ($\mathbf{x}$, $\mathbf{y}$)*-plane, **(e)**,**(k)** for the* ($\mathbf{y}$, $\mathbf{z}$)*-plane and **(f)**,**(l)** for the* ($\mathbf{x}$, $\mathbf{z}$)*-plane, for* $\mu_0 H = 1$ T *and* $\mu_0 H = 0.5$ T*, respectively. The transverse electric field* $E_{\mathrm{thermal,trans}}$ *(black squares) for all three geometries is displayed in panels **(g)**,**(m)** for the* ($\mathbf{x}$, $\mathbf{y}$)*-plane, **(h)**,**(n)** for the* ($\mathbf{y}$, $\mathbf{z}$)*-plane and **(i)**,**(o)** for the* ($\mathbf{x}$, $\mathbf{z}$)*-plane, for* $\mu_0 H = 1\,\mathrm{T}$ *and* $\mu_0 H = 0.5\,\mathrm{T}$*, respectively. The average sample temperature during these measurements was* $255\,\mathrm{K}$*. Red lines in the graphs are calculations based on our spin Nernst thermopower model via Eqs. (25),(26).*

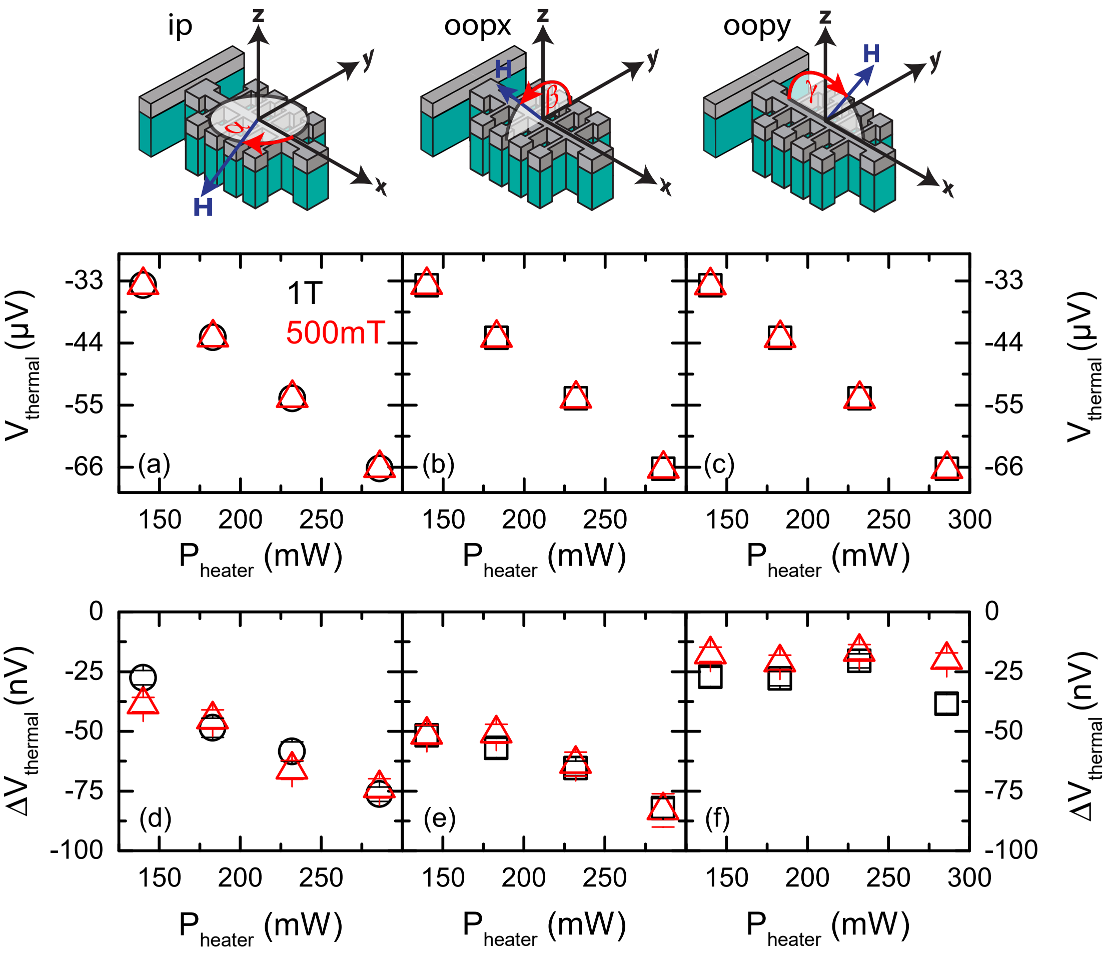


**Figure 7:** ***(a-c)*** *Power dependence of the thermal voltage* $V_{\text{thermal}}$ *and* ***(d-f)*** *the voltage modulation amplitude* $\Delta V_{\text{thermal}}$ *for ip (left column), oopx (middle) and oopy rotations (right column) at a base temperature of* $T = 220\,\text{K}$ *and magnetic field strength of* $0.5\,\text{T}$ *(red triangles) and* $1\,\text{T}$ *(black squares), respectively.*

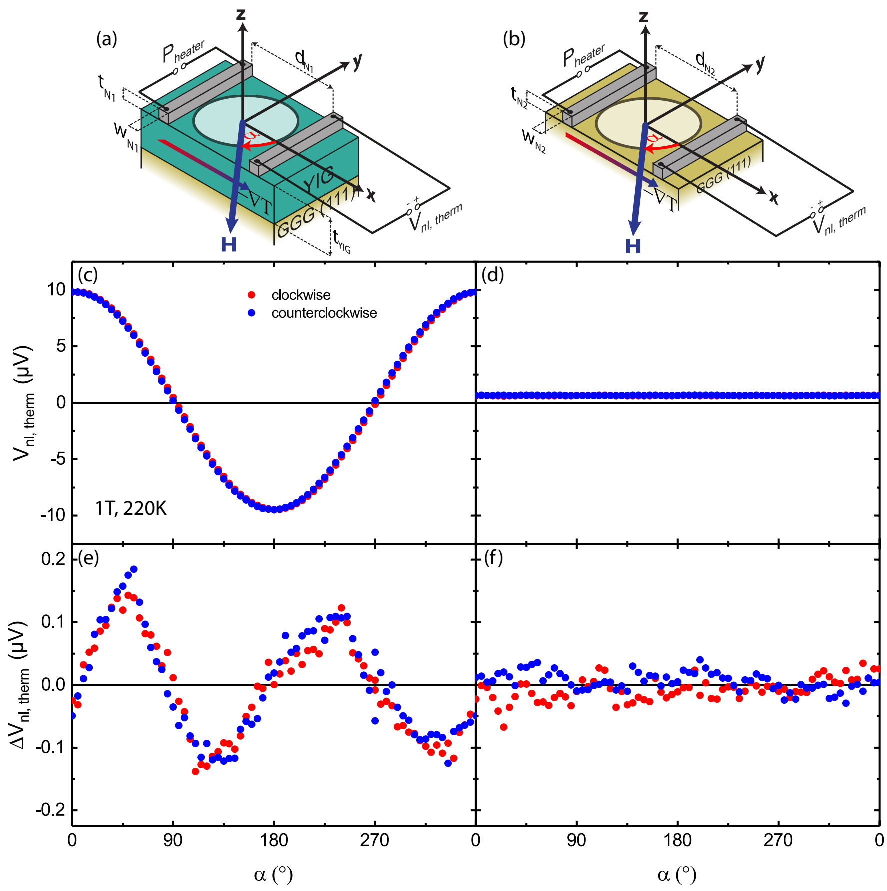


**Figure 8:** *Non-local thermopower signals for GGG/YIG/Pt and GGG/Pt samples.* ***(a)*** *sample sketch for the GGG/YIG/Pt heterostructure, with two Pt strips ($t_{N1}$ = 10 nm, $w_{N1}$ = 0.5 μm) separated by $d_{N1}$ = 1.6 μm.* ***(b)*** *GGG/Pt control sample with two Pt strips ($t_{N2}$ = 5.8 nm, $w_{N2}$ = 1 μm) separated by $d_{N2}$ = 2.6 μm.* ***(c)*** *Thermal voltage obtained for the GGG/YIG/Pt sample in the ip configuration. A sinusoidal signal is observed, which originates from the longitudinal spin Seebeck signal due to an out-of-plane temperature gradient.* ***(d)*** *Absence of an ip angular dependence of the thermal voltage in the GGG/Pt control sample.* ***(e)*** *Thermal voltage signal for the GGG/YIG/Pt sample after subtracting the spin Seebeck signal, which confirms the transverse spin Nernst magnetothermopower symmetry.* ***(f)*** *Thermal voltage signal for the GGG/Pt control sample shows* no angular dependence *even after subtraction of a constant voltage offset.*
